# Supplementary material for: Robust High-Resolution Video Matting with Temporal Guidance
Source: arXiv:2108.11515 source file (2021-08-25)
Supplement: Supplementary file 1 [file teaser.tex]

\includegraphics[width=\textwidth]{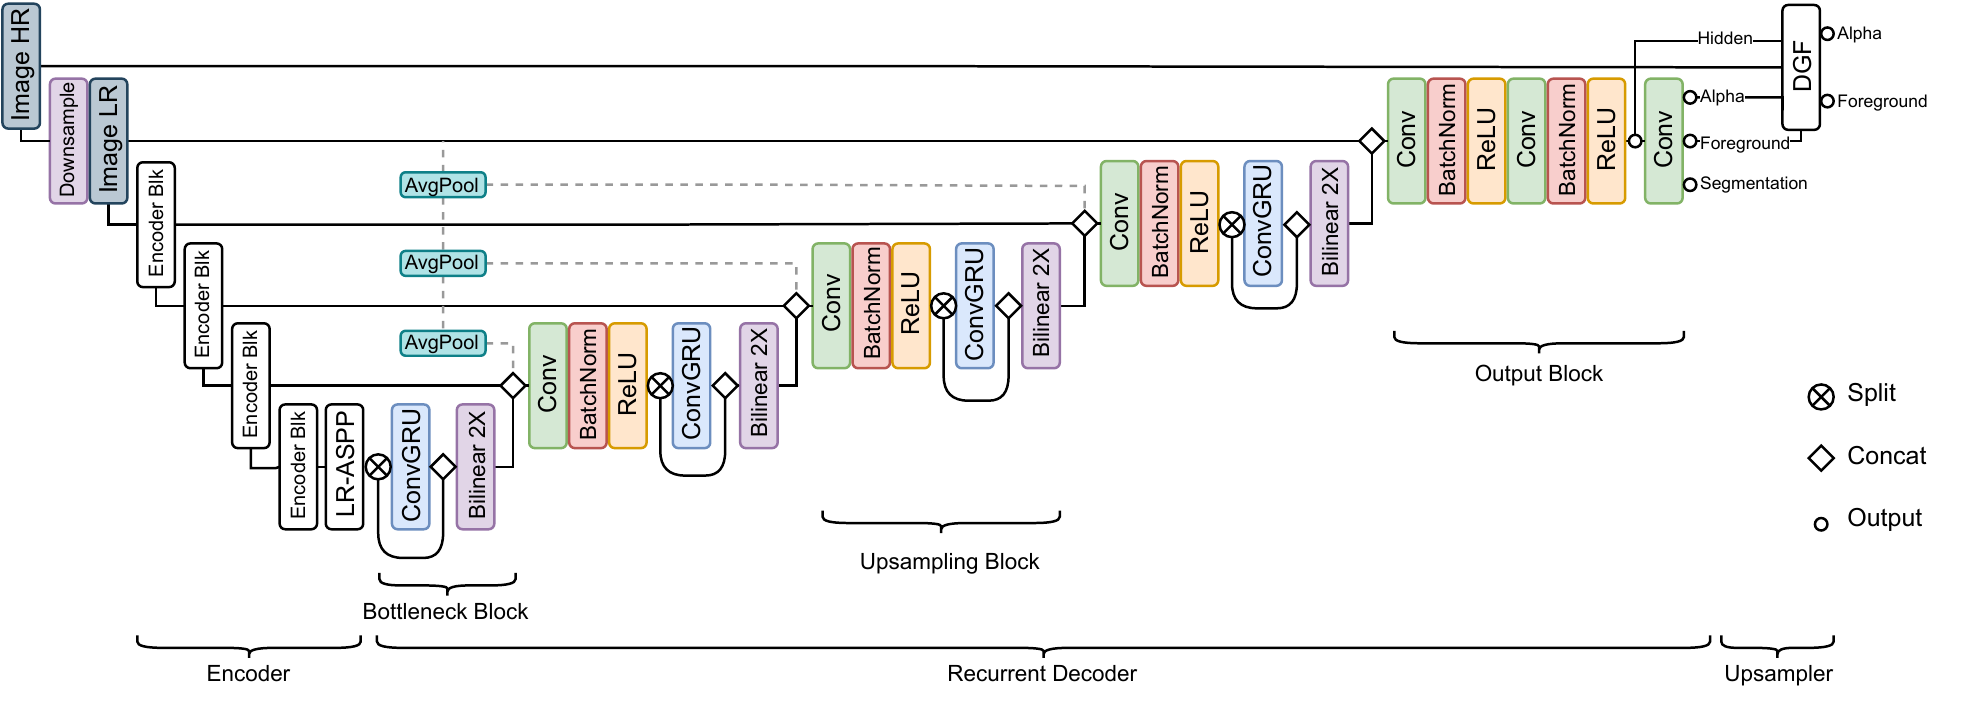}
\vspace{-18pt}
\captionof{figure}{Model architecture. The diagram is copied from the main text for reference. Our network consists an encoder that extracts individual frame's features, a recurrent decoder that aggregates temporal information, and a Deep Guided Filter (DGF) module for high-resolution upsampling. When processing high-resolution frames, the input is first downsampled to pass through the encoder-decoder network.}
